# Supplementary material for: Are Local Features All You Need for Cross-Domain Visual Place Recognition?
Source: arXiv:2304.05887 source file (2023-04-12)
Supplement: Supplementary file 1 [file supp1.tex]

TODO things for journal \\
- offline extraction (how Fig 1 changes when extraction of descriptors is done offline, and how much storage is required) \\
- more qualitative examples \\
- other methods like fire, how... \\
- considerations on hyperparams tuning \\
- perhaps tuning ransac threshold on sf-xl v2 for all methods, and see what happens \\

\section{Experiments}
In this Supplementary Material we report details that could not fit in the main paper.
In \cref{sec:further_qualitative} we provide further discussion to better understand strength and weaknesses of the tested methods.

\subsection{Additional qualitative results}
\label{sec:further_qualitative}
\myparagraph{Further analysis on computational cost}
In Fig. TODO we consider a scenario in which the extraction of local descriptors for the entire database of references images can be done offline. In general this entails heavy storage requirements that can be alleviated with the usage of quantization techniques \cite{Noh_2017_delf, Cao_2020_delg, Berton_2022_benchmark}. 
With respect to the analysis presented in the main paper, all the inference times are lower, and the relative relationships between methods are mantained as they all benefit from the offline extraction to some extent. This additional analysis gives a more complete picture of the costs that should be expected for real-world applications in which speed matters whereas storage is cheaply available.   

\myparagraph{SF-XL night errors correlation analysis}\\
We wanted investigate the behaviours of the considered models on the challenge posed by \textit{SF-XL test night} dataset. We have performed an exhaustive visual inspection of the failure cases of the considered models (SuperGlue, DELG and CVNet) for the queries for which the baseline provides at least a nominal positive reference \gba{add the number of cases}. We found that SuperGlue has some difficulties handling queries with repeated patterns and a major change in visual appearance at the same time, we guess it feels the lack of a global similarity based score in this cases. While DELG and CVNet sparingly fail on wide scenes representing multiple objects, where they occasionally retrieve a false positives that has the same spatial disposition of the query. In this scenario the weight of their global similarity score could be misleading and they feel the lack of highly optimized local features. Apart these considerations we found that the majority of the failures have no obvious human-eye pattern and that their errors are not mutually dependent. This is confirmed in \cref{fig:sfnight_correlation}, a correlation analysis between the rankings estimated by the considered methods shows that they are surprising weakly correlated if we consider that they achieves similar performance in the same task. Our conclusion is that the re-ranking methods reach comparable good performances following very different paths.

\begin{table}
\centering
\begin{adjustbox}{width=0.7\columnwidth}
\begin{tabular}{lcccc}
\toprule
\multirow{2}{*}{\begin{tabular}[c]{@{}c@{}}Re-ranking\\Method\end{tabular}} &
\multicolumn{2}{c}{Tokyo 24/7} \\
\cline{2-3}
& Day \#TP & Night \#TP \\
\hline
SuperGlue  & 101 & 100\\
DELG       & 101 & 100\\
LoFTR      & 101 & 98 \\
CVNet      & 101 & 101 \\
\bottomrule
\end{tabular}
\end{adjustbox}
\caption{\textbf{Tokyo day vs night.} Tokyo day and night top 1 analysis. We consider true positive and false positive for  the first scored references for day and night query pairs (100m treshold). We considered only query with a nominal positive reference for both cases night and day (103 over 105 pairs), we further removed night queries for which the positive reference was quite random with not visual clues. The models are shown quite roboust to night domain shift, in particular CVNet reaches its performance upper bound.\gt{perhaps it's better to express true positives in percentage}}
\label{tab:tokyo_day_night}
\end{table}

\begin{figure}
    \centering
\begin{tikzpicture}[scale=0.8]
  \foreach \y [count=\n] in {
       {1.00, 0.14, 0.10, 0.14, 0.13},
       {0.14, 1.00, 0.29, 0.31, 0.21},
       {0.10, 0.29, 1.00, 0.32, 0.24},
       {0.14, 0.31, 0.32, 1.00, 0.37},
       {0.13, 0.21, 0.24, 0.37, 1.00},
    } {
      %\ifnum\n<6
      %  \node[minimum size=6mm] at (\n, 0) {\n};
      %\fi
      % heatmap tiles
      \foreach \x [count=\m] in \y {
        \node[fill=yellow!\fpeval{100*\x}!purple, minimum size=8mm, text=black] at (\m,-\n) {\x};
      }
    }
  % column labels
      \foreach \a [count=\i] in {Cosplace,Superglue,LoFTR,DELG,CVNet} {
        %\node[minimum size=6mm] at (\i,0) {\a};
        \node[label={[rotate=-90, minimum size=6mm]\a }] at (\i-0.35,0+0.5) {};
        }
  % row labels
  \foreach \a [count=\i] in {Cosplace,Superglue,LoFTR,DELG,CVNet} {
    \node[minimum size=8mm] at (0-0.45,-\i) {\a};
  }
\end{tikzpicture}
  \caption{\textbf{SF-XL Night Spearman correlation matrix.} In the table are reported the correlation coefficients between the rank variables attributed by the models for all SF-XL queries. The model predictied ranks are only weakly correlated.}
    \label{fig:sfnight_correlation}
\end{figure}

% \begin{table}
% \begin{tabular}{ cc }   % top level tables, with 2 columns
% Superglue & LoFTR \\  
% % leftmost table of the top level table
% \begin{tabular}{ |c|c|c| } 
% \hline
% & DTP & DFP \\
% \hline
% NTP & 100 & 0  \\
% \hline
% NFP & 1 & 0   \\
% \hline
% \end{tabular} &  % starting rightmost sub table
% % table 2
% \begin{tabular}{ |c|c|c| } 
% \hline
% & DTP & DFP \\
% \hline
% NTP & 98 & 0  \\
% \hline
% NFP & 3 & 0  \\
% \hline
% \end{tabular} \\
% DELG & CVNet \\  
% % leftmost table of the top level table
% \begin{tabular}{ |c|c|c| } 
% \hline
% & DTP & DFP \\
% \hline
% NTP & 100 & 0  \\
% \hline
% NFP & 1 & 0   \\
% \hline

% \end{tabular} &  % starting rightmost sub table
% % table 2
% \begin{tabular}{ |c|c|c| } 
% \hline
% & DTP & DFP \\
% \hline
% NTP & 101 & 0  \\
% \hline
% NFP & 0 & 0   \\
% \hline
% \end{tabular} \\
% \end{tabular}
% \caption{\textbf{Tokyo day vs night.} Tokyo day and night top 1 analysis. We consider true positive and false positive for  the first scored references for day and night query pairs (100m treshold). We considered only query with a nominal positive reference for both cases night and day (103 over 105 pairs), we further removed night queries for which the positive reference was quite random with not visual clues. The models are shown quite roboust to night domain shift, in particular CVNet reaches its performance upper bound.}
% \label{tab:tokyo_day_night}
% \end{table}
