# Supplementary material for: Are Local Features All You Need for Cross-Domain Visual Place Recognition?
Source: arXiv:2304.05887 source file (2023-04-12)
Supplement: Supplementary file 2 [file supplementary.tex]

% % CVPR 2023 Paper Template
% % based on the CVPR template provided by Ming-Ming Cheng (https://github.com/MCG-NKU/CVPR_Template)
% % modified and extended by Stefan Roth (stefan.roth@NOSPAMtu-darmstadt.de)

% \documentclass[10pt,twocolumn,letterpaper]{article}

% %%%%%%%%% PAPER TYPE  - PLEASE UPDATE FOR FINAL VERSION
% \usepackage[review]{cvpr}      % To produce the REVIEW version
% %\usepackage{cvpr}              % To produce the CAMERA-READY version
% %\usepackage[pagenumbers]{cvpr} % To force page numbers, e.g. for an arXiv version

% % Include other packages here, before hyperref.
% \usepackage{graphicx}
% \usepackage{enumitem} % reduce space in enum
% \usepackage{amsmath}
% \usepackage{amssymb}
% \usepackage{booktabs}


% % It is strongly recommended to use hyperref, especially for the review version.
% % hyperref with option pagebackref eases the reviewers' job.
% % Please disable hyperref *only* if you encounter grave issues, e.g. with the
% % file validation for the camera-ready version.
% %
% % If you comment hyperref and then uncomment it, you should delete
% % ReviewTempalte.aux before re-running LaTeX.
% % (Or just hit 'q' on the first LaTeX run, let it finish, and you
% %  should be clear).
% \usepackage[pagebackref,breaklinks,colorlinks]{hyperref}


% % Support for easy cross-referencing
% \usepackage[capitalize]{cleveref}
% \crefname{section}{Sec.}{Secs.}
% \Crefname{section}{Section}{Sections}
% \Crefname{table}{Table}{Tables}
% \crefname{table}{Tab.}{Tabs.}


% %%%% added io
% % \usepackage[accsupp]{axessibility}  % Improves PDF readability for those with disabilities.
% \usepackage{multirow}
% \usepackage{rotating}
% \usepackage{adjustbox}
% \def\eg{\emph{e.g}\onedot} \def\Eg{\emph{E.g}\onedot}
% \def\ie{\emph{i.e}\onedot} \def\Ie{\emph{I.e}\onedot}
% \usepackage{mathtools}
% \usepackage{textcomp}
% \usepackage{gensymb}
% \usepackage{enumitem}

% \usepackage[dvipsnames]{xcolor}
% \newcommand*{\red}{\textcolor{red}}
% \newcommand*{\green}{\textcolor{green}}


% \newcommand{\gbe}[1]{{\color{teal}{[GBE:#1]}}}  %comment
% \newcommand{\gbet}[1]{{\color{teal}{#1}}} %coloured text
% \newcommand{\gt}[1]{{\color{orange}{[GT:#1]}}}  %comment
% \newcommand{\gtt}[1]{{\color{orange}{#1}}} %coloured text
% \newcommand{\cma}[1]{{\color{blue}{[CM:#1]}}}  %comment
% \newcommand{\cmat}[1]{{\color{blue}{#1}}} %coloured text
% \newcommand{\gba}[1]{{\color{cyan}{[GBA:#1]}}}  %comment
% \newcommand{\gbat}[1]{{\color{cyan}{#1}}} %coloured text
% \newcommand{\mmo}[1]{{\color{cyan}{[MM:#1]}}}  %comment
% \newcommand{\mmot}[1]{{\color{cyan}{#1}}} %coloured text

% \newcommand{\myparagraph}[1]{\vspace{4pt}\noindent\textbf{#1}}

% %%%%%%%%% PAPER ID  - PLEASE UPDATE
% \def\cvprPaperID{15} % *** Enter the CVPR Paper ID here
% \def\confName{CVPR}
% \def\confYear{2023}


% % questi packages servono per i tick e le x nella tabella dei datasets
% \usepackage{amssymb}% http://ctan.org/pkg/amssymb
% \usepackage{pifont}% http://ctan.org/pkg/pifont
% \newcommand{\cmark}{\ding{51}}
% \newcommand{\xmark}{\ding{55}}
% \newcommand\RX{\text{\red{\xmark}}}
% \newcommand\GT{\text{\green{\cmark}}}

% %%%%%%%%%%%%%%%%%%%%%%%%%%%%%%
% %alignment tables
% \usepackage{float}

% %figures
% \usepackage{tikz}

% \begin{document}

% %%%%%%%%% TITLE - PLEASE UPDATE
% \title{Are re-ranking methods robust to domain shift?\\Supplementary}

% \author{First Author\\
% Institution1\\
% Institution1 address\\
% {\tt\small firstauthor@i1.org}
% % For a paper whose authors are all at the same institution,
% % omit the following lines up until the closing ``}''.
% % Additional authors and addresses can be added with ``\and'',
% % just like the second author.
% % To save space, use either the email address or home page, not both
% \and
% Second Author\\
% Institution2\\
% First line of institution2 address\\
% {\tt\small secondauthor@i2.org}
% }
% \maketitle


% \input{chapters/supp1}


% %%%%%%%%% REFERENCES
% {\small
% \bibliographystyle{ieee_fullname}
% \bibliography{egbib}
% }

% \end{document}
